# Supplementary material for: Reconstructions of electron-temperature profiles from EUROfusion Pedestal Database using turbulence models and machine learning
Source: arXiv:2504.17486 source file (2025-04-24)
Supplement: Supplementary file 1 [file appendices.tex]

\section{Method for Integrating Temperature Profiles}\label{appendix:predictionMethods}

The results obtained in \cref{ssec:etaPredictions,ssec:alphaPredictions,sec:heuristicpred,} will, in general, begin by stating an explicit or implicit functional relationship between $\RLTe$ and $\RLNe$. Therefore, the starting point of our profile predictions is a differential equation of the form $\RLTe = f (*)$, or:
\begin{equation}\label{eq:dtdr}
	\der{T_e}{R} = - \frac{T_e}{R} f(*),
\end{equation}
where the $*$ represents the database parameters that are used for numerical integration and the numerical constants used for the function. These parameters may profile values, engineering parameters, or magnetic-equilibrium parameters.

Following \citet{Simpson_Separatrix}, the boundary condition for the integration is set as $T_e=100\;\mathrm{eV}$ at $\Rsep$, the radial location where $\psi_N = 1.0$, i.e., where the \fit $T_e$ profile itself has the value of $100\;\mathrm{eV}$, matching the separatrix heat-flux condition described in \cref{sec:geometry}. The numerical integration is then carried out inwards from the position of the separatrix, spanning the interval where the pedestals normally lie. Once a predicted profile has been computed for each pulse, a new $\mtanh$ profile is fit to the prediction, and the resulting parameters are compared to the parameters that are contained in the original database, i.e., to the $\mtanh$ parameters of the $\fit$ profile.

\subsection{Finding Best-fit Parameters}\label{appendix:bestFit}
In order to identify the best-fit parameters for a certain scaling (e.g. identifying an $\eta_e$ in \cref{eq:etaDefinition} which produces an optimal prediction) is carried out by minimising the absolute difference between the $\fit$ $T_e$ profile and the reconstructed $T_e$ profile over some radial domain $\mathcal{D}$. $\mathcal{D}$ can represent a full-pedestal interval encompassing the core slope ($\psi_N \in [0.85,1.0]$), or any region in the pedestals (represented by some sub-interval of $\psirenorm \in [0,2]$). This means that the optimal parameters can be found to match the pedestal region, or an overarching section of the pedestals in order to produce good $\mtanh$ parameters as benchmarks for the fit. The optimization and integration is done in real space, but for consistency, we use $\psi_N$ intervals to denote locations.

Minimising the residual $\Delta$ between the $\fit$ $T_e$ profile and the reconstructed $T_e$ profile viz.:
\begin{equation}
	\Delta = \int_{\mathcal{D}} \mathrm{d} R \left(T_{e,\fit}-T_{e,\mathrm{Rec}}\right)^2
\end{equation}
is equivalent to minimizing a weighted difference between the $\fit$ $\RLTe$ and the reconstructed $\RLTe$: a local inaccuracy of $\RLTe$ does not have a clear consequence on the accuracy of the $T_e$ profile prediction, as can be inferred from \cref{fig:ETGparamScan} in \cref{appendix:etgparamscans}.

\section{Sensitivity of ETG-Heat-Flux Models to Parameters} \label{appendix:etgparamscans}

In \cref{sec:heuristicpred}, we describe the results of adopting a heat-flux scaling of the form given in \cref{eq:HeatFluxA} across the entire pedestal profile, with constant parameters $A$, $\etacr$, and $\beta$. Additionally, the other available and implicitly chosen parameters in this model are the separatrix position $\Rsep$ and the electron-temperature at the separatrix $\Tesep$. These are used as the boundary conditions for the integration of profiles. In order to maintain consistency with the experimental data available, the separatrix location and temperature will be treated as a single parameter such that the profiles are integrated beginning from a certain initial radial location $R_{\mathrm{init}}$, and electron-temperature, $T_{e,\mathrm{init}}$ is that of the $\fit$ profile at $R_{\mathrm{init}}$. 
All possible models which determine $\RLTe$ as a function of local parameters of the profile will integrate to the exact same profile irrespective of the initial conditions $R_{\mathrm{init}}$ and $T_{e,\mathrm{init}}$ as long as they pass through the same $(R,T_e)$ \quotemarks{pair} at any $R$. Nominally, for \cref{sec:heuristicpred},  $T_{e,\mathrm{init}} = \Tesep = 100\;\mathrm{eV}$. 

% in models where \RLTe is obtained from a scaling law which the electron-temperature does not appear explicitly, the resulting integrated profiles are identical up to a multiplicative factor which can be fixed by matching the separatrix temperature. For the current models, the existence of $Q_{e,GB}$ in the normalisation of the heat fluxes means that the profiles are meaningfully different based on the initial condition. Nonetheless, two different integrated profiles will integrate to the same shape as long as they pass through the same $(R,T_e)$ point, irrespective of the local heatflux model used. This further justifies the choice to have $R_{init}$ and $T_{e,init}$ as determined together

\begin{figure}%[t]
	\centering
	\includegraphics[width=\textwidth]{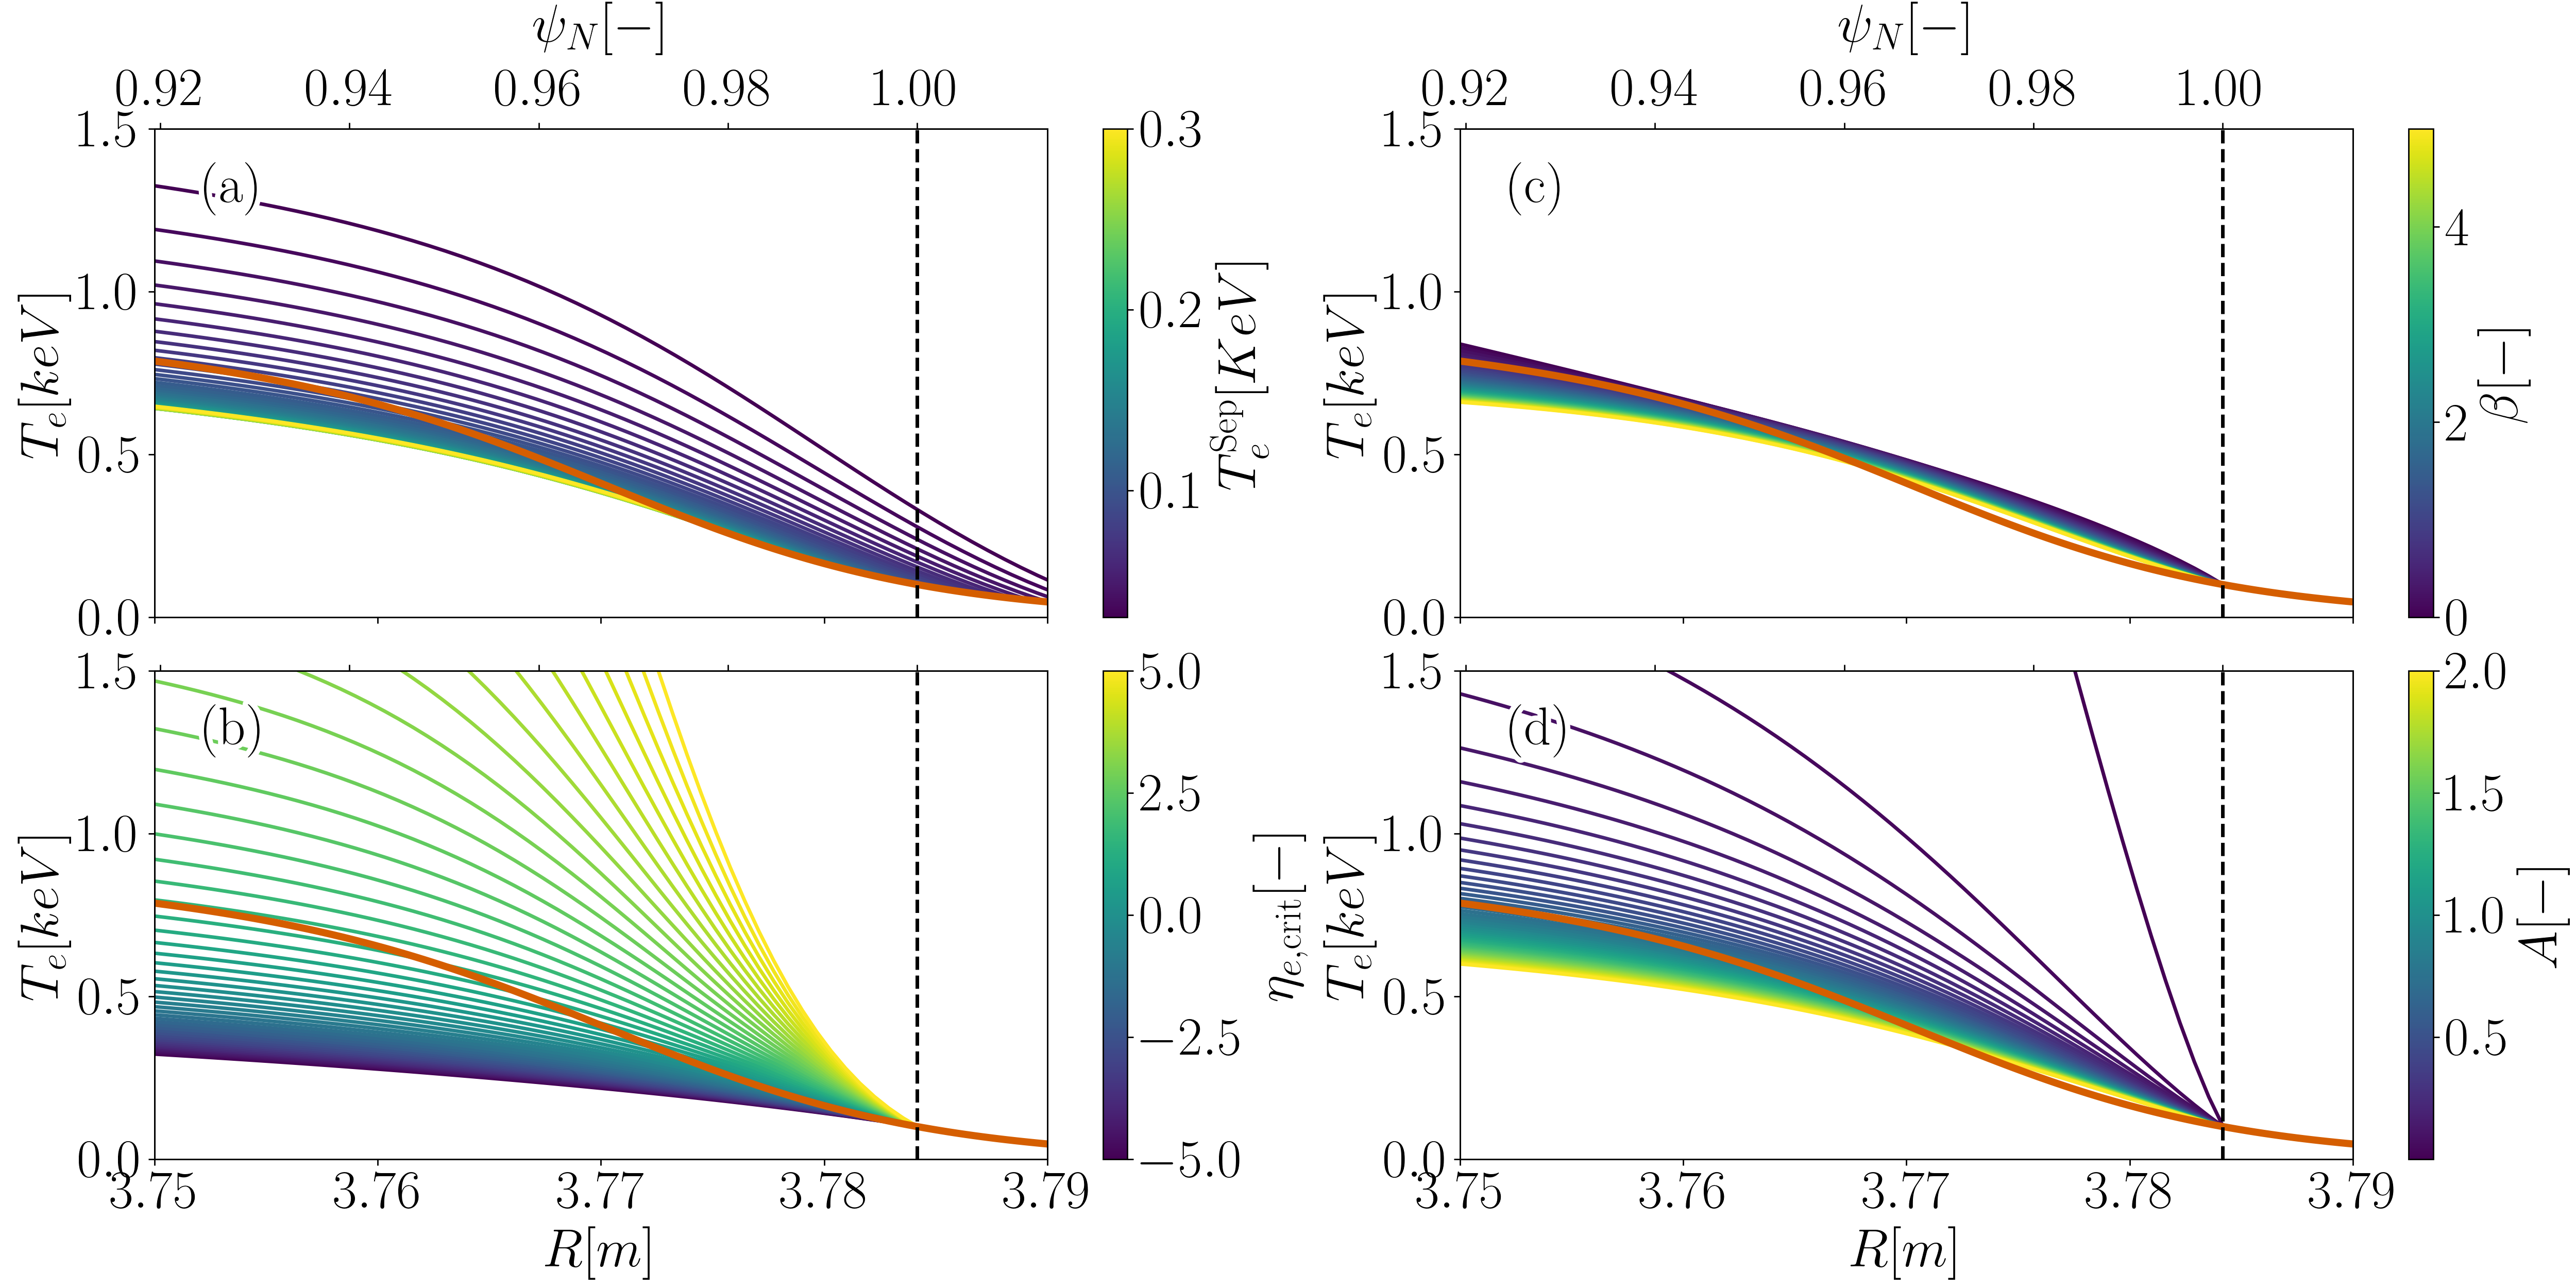}
	\caption{\centering  {\fit $T_e$ profiles of pulse $\examplepulse$ are shown in orange, compared with ETG profiles integrated from an initial electron temperature $T_{e,\mathrm{init}}\equiv \Tesep$. Each figure contains variations of one of the parameters used in heat-flux model in \cref{eq:HeatFluxA}: (a) $T_{e,\mathrm{init}}$, (b) $\eta_e$, (c) $\beta$, (d) $A$ while keeping the other parameters at the nominal values of \cref{eq:HeatFluxA}. The vertical dashed lines represent the location of the conventional separatrix location at $T_e=100\; \mathrm{eV}$.}}
	\label{fig:ETGparamScan}
\end{figure}

The predictions using models in \cref{eq:HeatFluxA} and \cref{eq:HeatFluxB} are very similar for the whole database. It is therefore important to discuss the sensitivity of the prediction to the exact value of $T_{e,\mathrm{init}}$ and the values of the heat-flux scaling parameters $A$, $\etacr$, and $\beta$, in order to understand the robustness of the prediction. \cref{fig:ETGparamScan} displays the results of scans in each of the free parameters.

The model is very stable to changes in $A$ and $\beta$. Variations in $A$ are equivalent to adjustments to the local heat flux (or the gyro-Bohm heat flux normalisation), affecting the overall size of \RLTe. Changes in $\beta$ adjust the position of the pedestal top, alongside affecting the profile's behaviour beyond the pedestal top. High values of $\beta$ are equivalent to \quotemarks{clamping} $\RLTe$ to $ \etacr \times \RLNe$, whereas low values of $\beta$ reduce the importance of $\RLNe$.
The profiles in this scan are insensitive to increases of $T_{e,\mathrm{init}}$ as a result of the fact that at nominal values of  $A$, $\etacr$, and $\beta$, the prediction approximates the \fit profile well. Reductions of $T_{e,\mathrm{init}}$ result in large displacements of $R_{\mathrm{init}}$, causing high differences in the prediction.

The value of $\etacr$ changes the predictions most significantly over an order-unity variation in the parameter. $\etacr$  introduces an effective minimal limit on \RLTe in order to keep the term $\eta_e - \etacr$ positive, or, physically, to maintain the turbulence in a supercritical regime. Explicitly, increases in $\etacr$ cause the normalised temperature gradient $\RLTe$ to increase in order to satisfy the heat-flux equation imposed on the profile. This means that the predicted temperature at the top of the pedestal is increased. In spite of the increased relevance of $\etacr$, the two models used in \cref{sec:heuristicpred} lack a significant difference in any of the parameters in the integration. This justifies the similarity between the prediction benchmarks in \cref{fig:EtgResults}.

\section{Neural Networks and Methods}\label{appendix:neuralnets}

This appendix details the machine-learning methods used to reconstruct $T_e$ in our database. These methods include the usage of data selection, processing, and augmentation, alongside choosing training strategies and network architecture.

\subsection{Data Selection and Pre-processing} \label{sappendix:preprocessing}

The database we use includes parameters associated with each pulse, which can be real-valued (any database parameter or profile) or discrete \quotemarks{qualifiers} (the strike-point configuration). Categories are treated separately, and we also make a distinction between the preparation of database parameters and database profiles. The aim of our data processing is to translate the data to a series of scalars which can be assembled into a structured vector describing the pulse. 

The discrete-valued strike points are one-hot encoded to a 6-dimensional vector which contains a value of $1$ in a location corresponding to each of the 6 combinations of strike points in the database.

The $n_e$ and $T_e$ profiles are sampled from \fit profiles at $64$ equally-spaced radial locations which are chosen to be common across the database. The radial locations are chosen in the $R$ coordinate, spanning between $R=3.7\;\mathrm{m}$ and $R=3.85\;\mathrm{m}$, which includes all of the pedestals in the database. The choice of $R$ as opposed to $\psi_N$ or $\psirenorm$ is made in order to avoid the inclusion of data which is aware of the pedestals - $\psi_N$ contains information obtained from equilibrium reconstructions of the plasma profiles, and $\psirenorm$ makes use of the pedestal-top locations.

Where available, experimental uncertainties are also included for the purpose of augmentation. \fit profiles contain, by default, uncertainties derived from the \mtanh fits, however we aim to include locally relevant experimental uncertainties. For this, the experimental errors included in \raw profiles are processed to be sampled at the same $64$ radial locations. The values of the experimental errors are convolved with a Gaussian kernel of a full-width-half-maximum which matches the instrument function of the HRTS diagnostic \citep{Frassinetti_MeasurementMethods}, and then are passed through a low-pass filter to obtain good numerical interpolation. The convolved and filtered experimental errors offer an excellent estimate for the mean uncertainties at each location. The interpolation method used allows us to sample these mean errors at each radial location used for the profiles.

\subsection{Augmentation} \label{sappendix:augmentation}

Augmentation is essential for the training stability and convergence of neural networks, and it plays an important role in transforming the limited database of $1251$ pulses into a statistically meaningful training set. It is also important to introduce awareness of the experimental uncertainties into the neural networks in order to allow for correct interpolation and weighing of the experiments based on their accuracy.

\begin{figure}%[t]
	\centering
	\includegraphics[width=\textwidth]{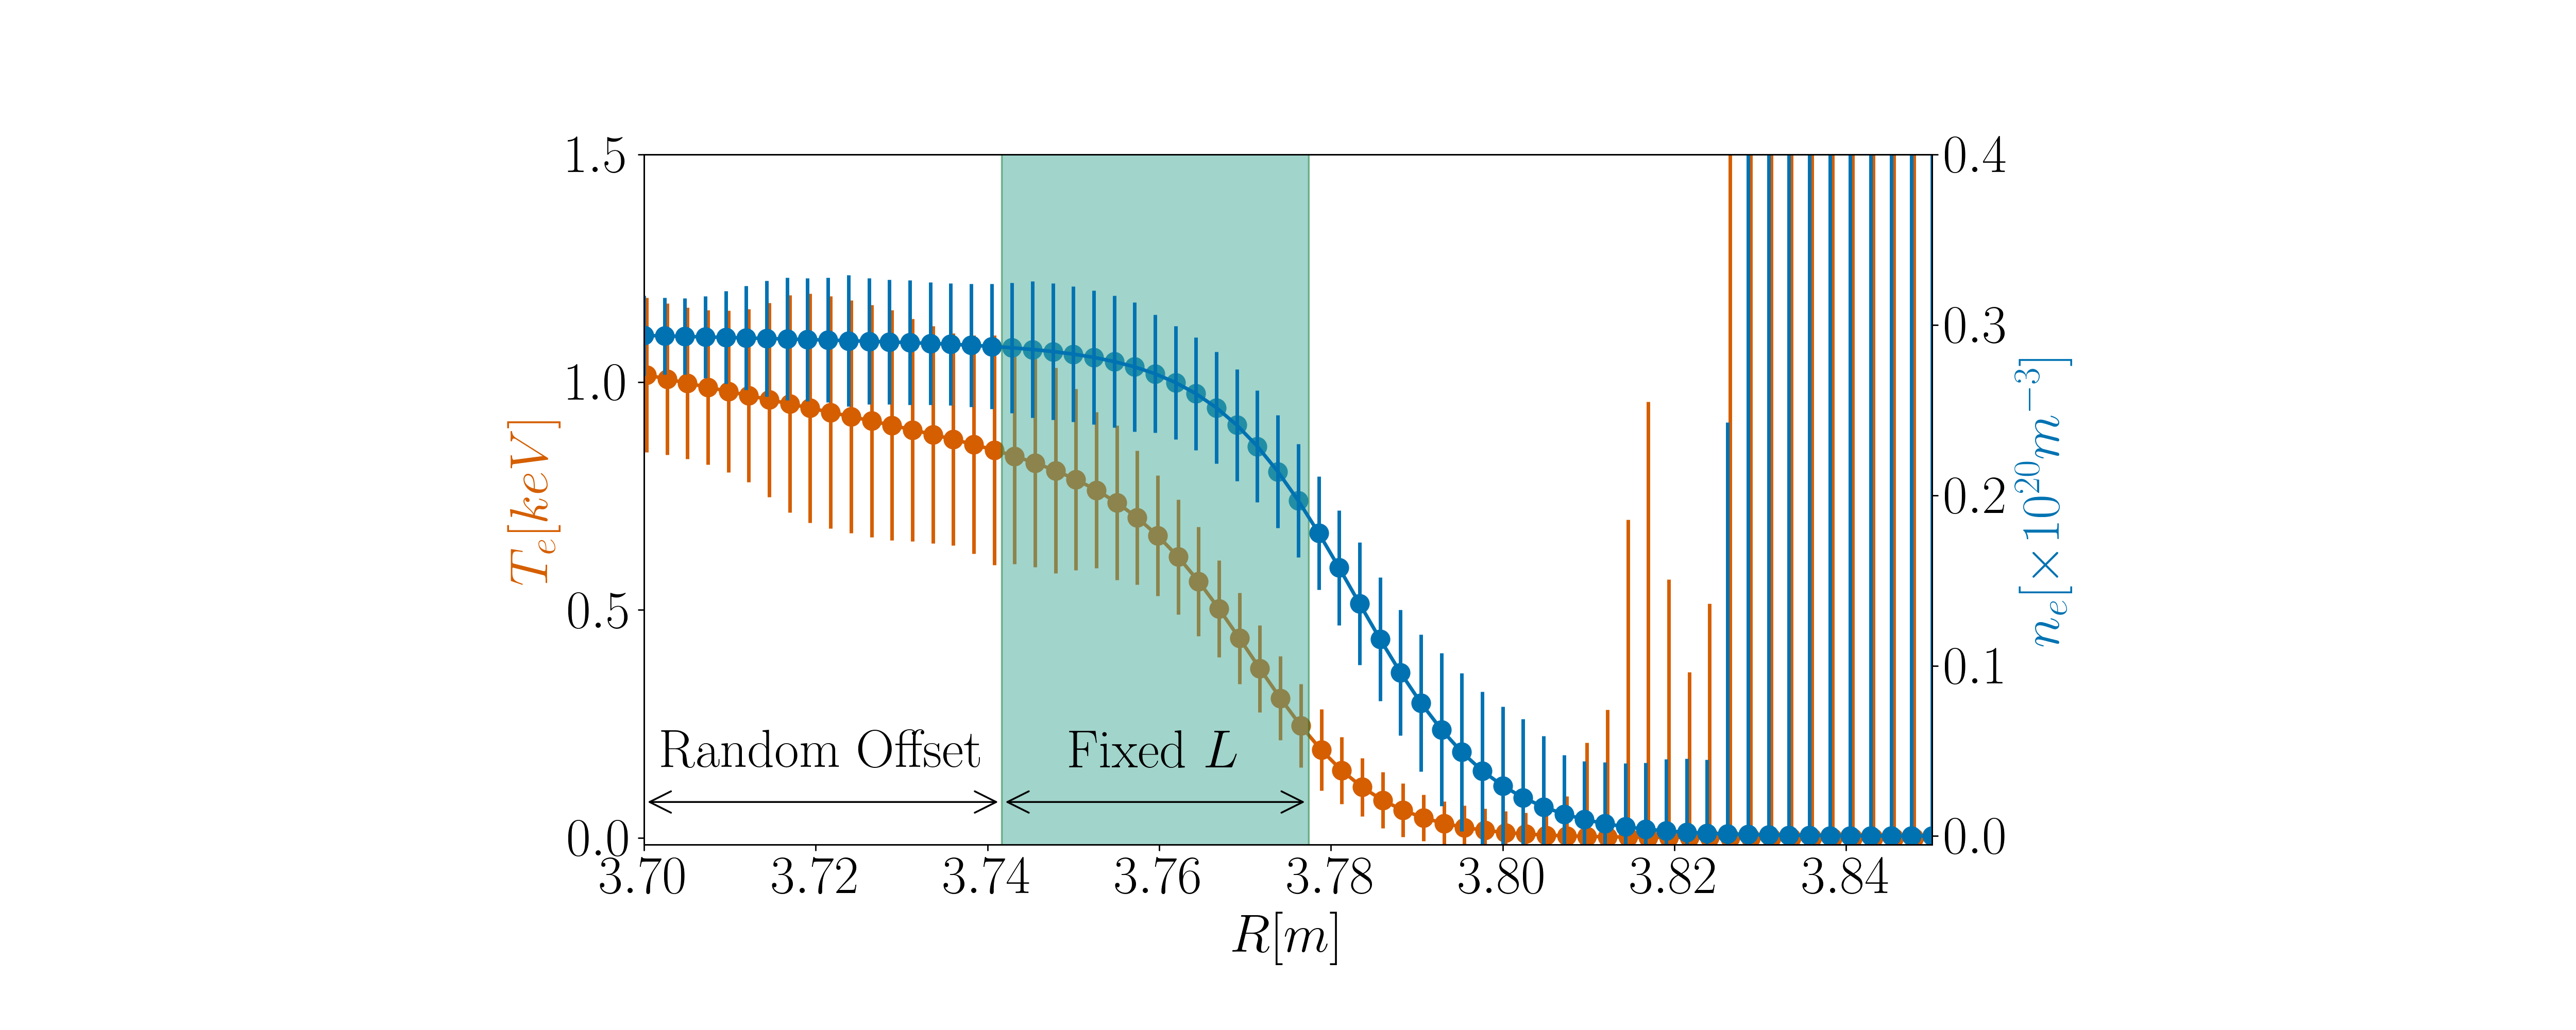}
	\caption{\centering  {The $n_e$ (blue) and $T_e$ (orange) profiles of pulse $\examplepulse$, with $64$ numerical samples at equally spaced radial locations. The error bars represent the associated convolved and low-pass-filtered experimental uncertainties, as described in \cref{sappendix:preprocessing}. The green box represents a subset of $L$ consecutive numerical values. The beginning location of the subset is chosen randomly as part of the augmentation process described in \cref{sappendix:augmentation}.}}
	\label{fig:randomCrop}
\end{figure}

For the purpose of assembling the inputs, each separate piece of information is comprised of $N$ different parameters and several profiles of $L$ values at different positions assembled into a vector. The pulses are therefore treated as populating an $N$-dimensional parameter space, for which the parameter-space density is calculated using a Gaussian-kernel-density-estimator. Using the parameter-space density at the mean values of the parameters associated to each pulse, an augmentation number is calculated in order to compensate for over-population or under-population of the parameter space. This results in a training dataset in which the pulses in sparse regions of the parameter space are represented by more augmented entries, while the pulses in the dataset in densely populated regions of the parameter space are represented by fewer pulses. The profiles included in training are computed by taking randomly-positioned subsets of $L$ consecutive values of the profiles of $T_e$, $n_e$, $\psi_N$, and $R$, as depicted in \cref{fig:randomCrop}. The random positioning of the subsets helps the networks match the features of the profiles to the prediction, as opposed to an inflexible memorisation based on the exact radial location of each numerical value. Including $R$ and $\psi_N$ in the networks also allows to test the importance of the location to the prediction.

All resulting augmented entries of the dataset (parameters and profiles) also include Gaussian random noise which matches the experimental uncertainties of each pulse. This synthetically generated dataset statistically exactly matches each of the original pulses, except that it is spread more uniformly across the parameter space. Furthermore, the networks are more capable to perform a correct interpolation in our parameter space if they are exposed during training to noisy data which matches experimental uncertainties.

\subsection{Normalisation and Loss}

These augmentation techniques result in a dataset comprised of many vectors which contain the concatenated parameters and profile values. For numerical stability, all of the values in these vectors are normalised post-augmentation. Slight performance differences are found when performing a linear normalisation to the $0-1$ interval or a normalisation to a mean of $0$ or a standard deviation of $1$. The normalisation choice is only relevant to the training hyperparameters of the networks such as the optimizer used or the learning rate as numerical instability can sometimes arise.

In order to train the neural network, a mean-squared loss is used. The normalisation affects the exact value of the loss function when presented for the parameter combination scans.

\subsection{Train-Test Split}

We use a randomized $80\%-20\%$ train-test split, i.e. $1000$ pulses are used for the training of the neural networks and $251$ pulses are used for testing the accuracy of predictions. Parameter-space densities and normalisations are calculated using exclusively the $1000$ training pulses. These parameter-space properties are then used to augment both the training $1000$ pulses as well as the $251$ test pulses. All test pulses have identical augmentation numbers in order to avoid biasing the performance assessment of the networks, whereas the augmentation of the test pulses aims to reduce the variations in parameter-space densities.

\subsection{Neural Network Architecture}

We use a simple feed-forward neural network with $6$ linear layers and $5$ rectified linear units (ReLU) layers. The input and output sizes of the linear transformations are chosen to match the dimensions of the input and output based on the profiles and parameter combinations in the dataset, whereas the hidden sizes are chosen to be $128$ which provide ample ability to capture the trends in the data while reducing overfitting. Dropout layers are sometimes included to reduce overfitting. %For the predictions of the separatrix loss power, $P_{Sep}$, dropout layers are also included to reduce overfitting. - this requires a bit more info

% a few things one would like to include in the final version for the thesis:
% we discard profiles with a minimum amplitude. this is to reduce the amount of zero input-> finte output sets which mess up the training
% the exact values of augmentation vary - the network manages to act as a de-noiser on top of everything else, successfully predicting the average output - when the learning rate is too low the validation error increases resulting in fitting noise; when the learning rate is high, the networks are unstable

%we tried using psep and it semi failed and semi worked
